# Supplementary material for: Federated Document Visual Question Answering: A Pilot Study
Source: arXiv:2405.06636 source file (2024-05-22)
Supplement: Supplementary file 1 [file supp.tex]

% \clearpage
\newpage
\appendix
% make all tables and figures in appendix with A.1, A.2...
\setcounter{figure}{0}

\setcounter{table}{0}

\setcounter{equation}{0}

\section{Dataset}\label{sec:supp_dataset}
Figure \ref{fig:data_partition} illustrates data populations resulted from our partitioning scheme.
\begin{figure}
\begin{subfigure}[h]{0.483\linewidth}
\includegraphics[width=\linewidth]{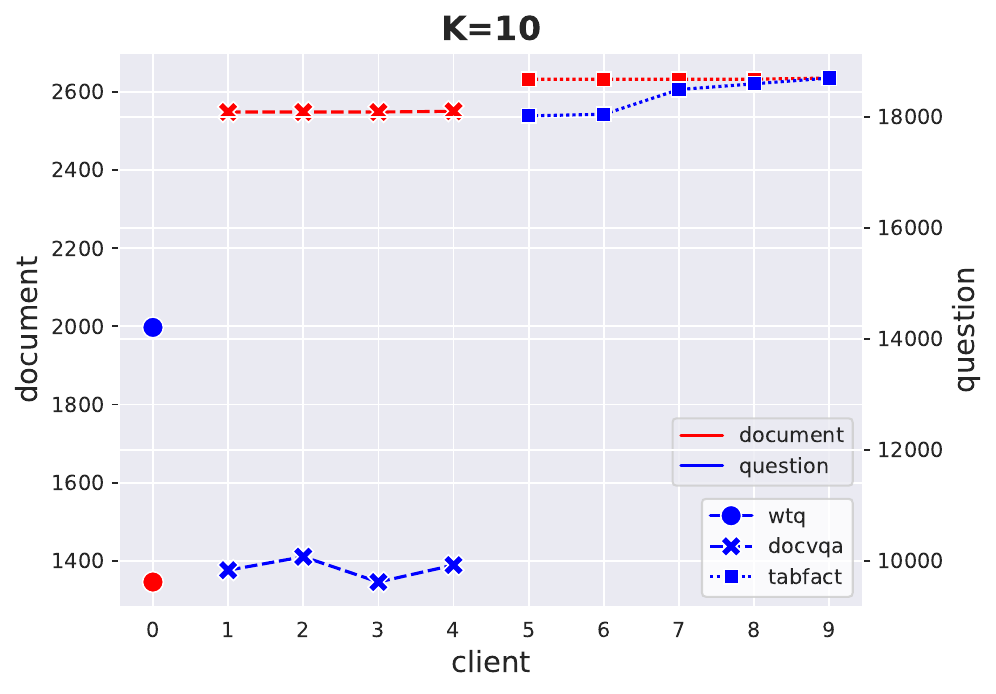}
\end{subfigure}
% \hfill
\begin{subfigure}[h]{0.48\linewidth}
\includegraphics[width=\linewidth]{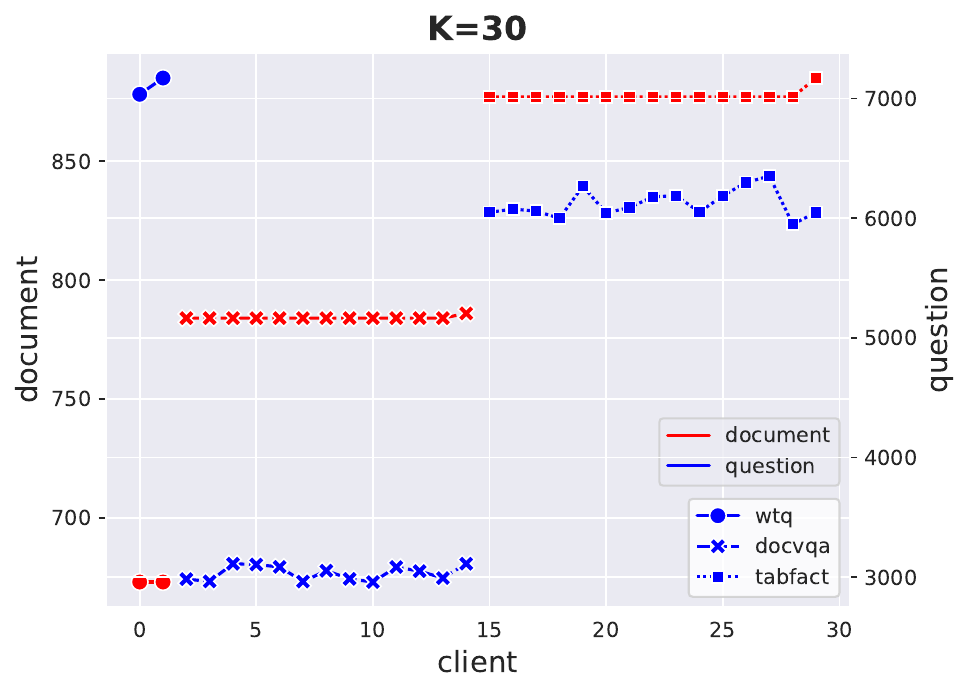}
\end{subfigure}
\caption{\textbf{Statistics} on the number of training documents/questions each client holds in our partition scheme.}
\label{fig:data_partition}
\end{figure}

\section{More on Ablation Study}\label{sec:supp_dataset}
